# Supplementary material for: OmniLabel: A Challenging Benchmark for Language-Based Object Detection
Source: arXiv:2304.11463 source file (2023-08-14)
Supplement: Supplementary file 1 [file supp_overview.tex]

\section{Overview of Appendix}

\begin{itemize}
    \item \textbf{\cref{sec:supp_data_analysis}:} Additional analysis of the OmniLabel dataset
    \item \textbf{\cref{sec:supp_data_collection}:} Additional information on data collection
    \item \textbf{\cref{sec:supp_code_and_dataset}:} Code and mini-dataset
    \item \textbf{\cref{sec:supp_dataset_examples}:} Visualizations of the OmniLabel dataset
\end{itemize}
